# Supplementary material for: Congestion-aware Routing and Rebalancing of Autonomous Mobility-on-Demand Systems in Mixed Traffic
Source: arXiv:2003.04335 source file (2020-03-09)
Supplement: Supplementary file 1 [file 99_Appendix.tex]

\section{Appendix} \label{sec:appendix}
\subsection*{A. Description of datasets} \label{app-sec:description-dataset}
\subsubsection*{1) Eastern Massachusetts Area (EMA)}
The Boston Region Metropolitan Planning Organization (MPO) provided access to two datasets of the EMA network:  \noindent (1) A dataset which contains the average speed for every minute of the year 2012 and 2015 for more than 13,000 road segments (see Fig.~\ref{fig: EMA_net}). For each road segment, we have access to information about instantaneous, average, and free-flow speeds (in \emph{mph}), date, time, and travel time (in \emph{minutes}). \noindent (2) A flow capacity (in \emph{vehicles per hour}) dataset which includes capacity data for more than 100,000 road segments. For more detailed information of the two datasets, see \cite{Zhang2016}.

\subsubsection*{2) New York City (NYC)} 
We built the NYC transportation network through two open source datasets: \noindent (1) OpenStreetMaps (OSM) \cite{OpenStreetMap} from where we retrieved the network topology and road characteristics of NYC and \noindent (2) the \emph{Uber Movement Speed Dataset} \cite{UberData} which provides average speeds of road segments on an hourly basis and which can be easily matched with OSM network.

\subsection*{C. Preprocessing} \label{app-sec:preprocessing}
\begin{itemize}
  \item[1)] \textit{Selecting a sub-network:}  \label{app-subsec:selecting subnet}
    \begin{itemize}
      \item[-]{\textit{EMA: }}
      To mitigate the computational complexity while still capturing the key elements of the EMA network, we considered a representative highway sub-network (Fig.~\ref{fig: EMA_net}) where there are 701 road segments, composing a road network with 8 nodes and 24 links. This links and nodes compose a road network $\big( {\tilde {\scrV},\tilde {\scrA}}, \tilde {\scrW} \big)$. Every node in the network is also considered as a zone (Origin-Destination candidate).
      \item[-]\textit{{NYC: }}
      Similar to EMA but in an urban environment we sought to reduce the dimensionality of the full network (Fig.~\ref{fig:NYC_full_net}). To do this, we first select the a subset of nodes from the full network to be the nodes of the sub-network ans create edges between these nodes. We chose the subset of nodes in a way that matched our knowledge of the connectivity of NYC network. Then, for each edge connecting the sub-network nodes, we solve a shortest path problem on the full network and report the travel time as the travel time in the smaller network. Finally, we select some of the nodes to serve just as intersections, and other to be Zones. See Fig.~\ref{fig:NYC_net} where the bubbled nodes we considered as zone nodes. 
    \end{itemize}

\item[2)] \textit{Calculating average speed and free-flow
    speed:} \label{app-subsec:avg-speed}

  We choose a time instances set $\scrT$ consisting of a set of
  minutes or hours (for EMA and NYC, respectively) of a time period of interest and calculate the average speed for each road segment.
  We match these values with the capacity dataset. Then, for each road segment we compute a proxy of the
  \textit{free-flow speed} by using the 85th-percentile of the
  observed speeds on that segment.
   
\item[3)] \textit{Aggregating flows of the segments on
    each link:} \label{app-subsec:aggreggating-flows}

  For $i \in [\kern-0.15em[ \tilde\scrA ]\kern-0.15em]$, let $\{
  {v_i^{{j}}},{t_i^{{j}}},{v^{{0j}}_i},{t^{{0j}}_i},{m_i^{{j}}}; \, j =
  1, \ldots, J_i \}$ denote the available observations ($v_i^{{j}}$,
  $t_i^{{j}}$), and parameters ($v^{{0j}}_i$, $t^{{0j}}_i$, $m_i^{{j}}$)
  of the segments composing the $i$th \textit{physical} link, where, for
  each segment $j$, $v^{{j}}_i$ (resp., $v^{{0j}}_i$) is the
  \emph{average speed} (resp., \emph{free-flow speed}; in \emph{miles
    per hour}), $t^{{j}}_i$ (resp., $t^{{0j}}_i$) is the \emph{travel
    time} (resp., \emph{free-flow travel time}; in \emph{hours}), and
  $m_i^{{j}}$ is the \emph{flow capacity} (in \emph{vehicles per
    hour}). Then, using Greenshield's model \cite{Greenshields1935}, we calculate the
  \textit{traffic flow} (in \emph{vehicles per hour}) on segment $j$ by
\begin{align}
{\hat x_i^{{j}}} = \frac{{4{m_i^{{j}}}}}{{{v^{{0j}}_{i}}}} {v_i^{{j}}} - \frac{{4{m_i^{{j}}}}}{{(v^{{0j}}_{i})^2}} (v_i^{{j}})^2.
\label{Gr}
\end{align}
In our analysis, we enforce ${v_i^{{j}}} \leq
v_i^{{0j}}$ to make sure that the flow given by \eqref{Gr}
is non-negative. In particular, if for some time instance
${v_i^{{j}}} > v_i^{{0j}}$ (this rarely
happens), we set ${v_i^{{j}}} =
v_i^{{0j}}$ in \eqref{Gr}, leading to a zero flow
estimation for this time instance.
Aggregating over all segments composed of link $i$ we compute:
\[
\hat x_i = \frac{{\sum\nolimits_{j = 1}^{J_i}
        {{\hat x_i^{{j}}}{t_i^{{j}}}}
}}{{\sum\nolimits_{j = 1}^{J_i} {{t_i^{{j}}}}
}},\,\,
{t_i^{{0}}} = \sum\nolimits_{j = 1}^{J_i}
{{t^{{0j}}_{i}}},\,\,
{m_i} = \frac{{\sum\nolimits_{j = 1}^{J_i}
        {{m_i^{{j}}}{t^{{0j}}_{i}}}
}}{{\sum\nolimits_{j = 1}^{J_i} {{t^{{0j}}_{i}}} }},  
\]
where $\hat x_i^j$ is given by \eqref{Gr} and ${t^{{0j}}_{i}} =
v_i^{{j}} t_i^{{j}}/v^{{0j}}_{i}$,
$j = 1, \ldots ,J_i$.

\end{itemize}

\begin{figure}[ht]
    \centering
    \begin{subfigure}{0.59\linewidth}
        %\centering
        \includegraphics[width=\linewidth]{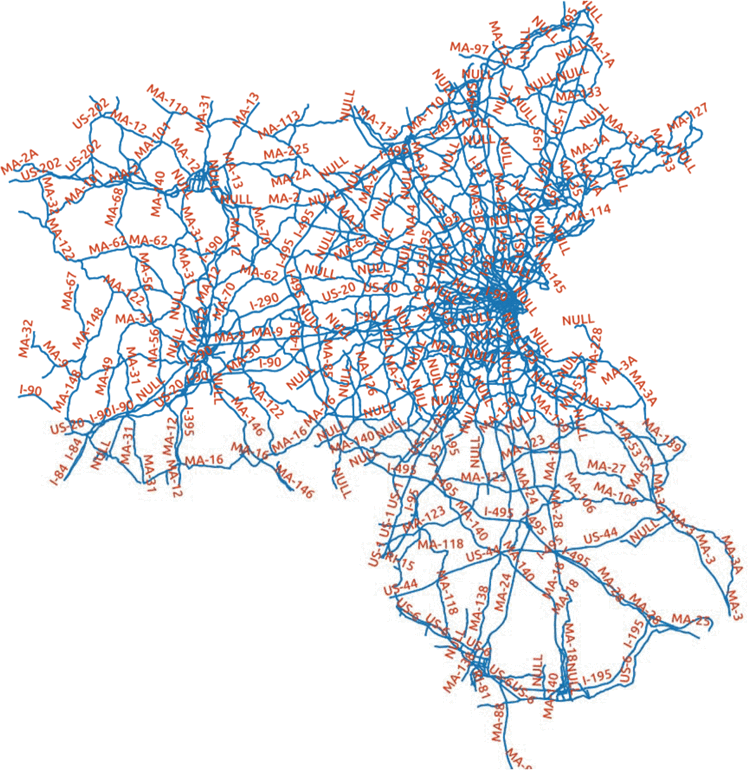}
        \caption{}
        \label{fig: EMA_net}
    \end{subfigure}
    \begin{subfigure}{0.39\linewidth}
        \centering
        \includegraphics[trim={0 0 0 0},clip, width=\linewidth]{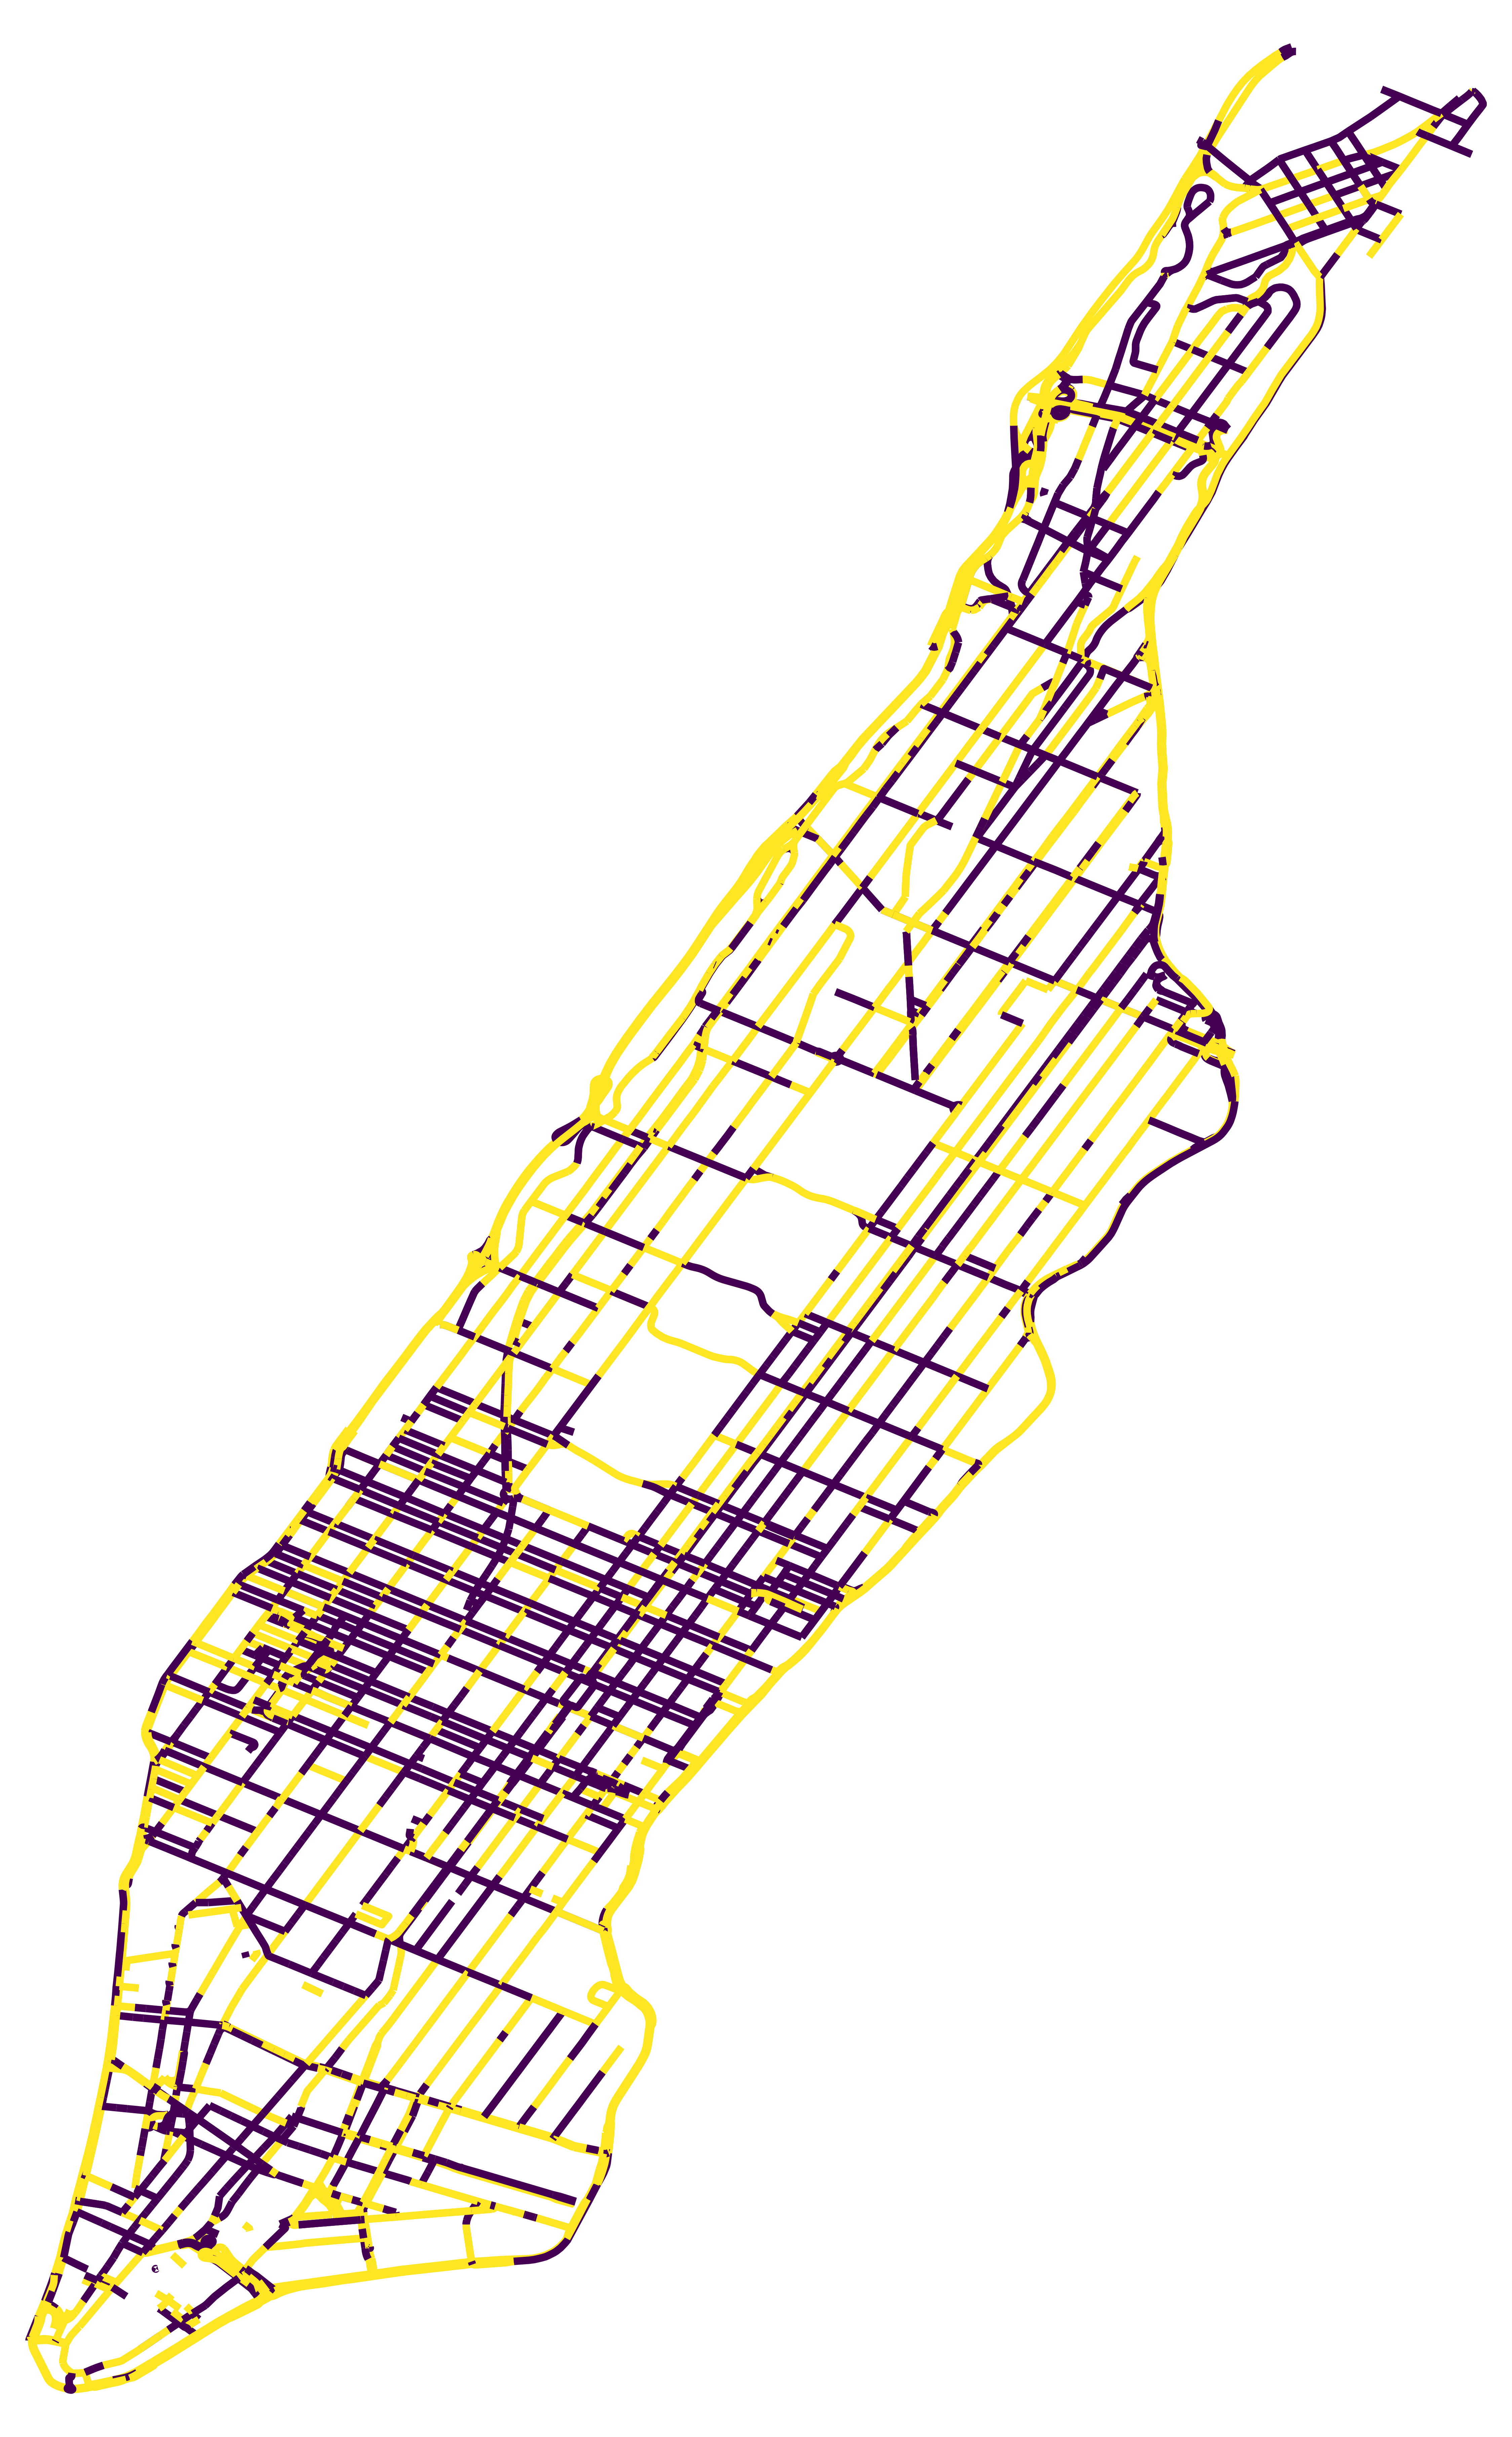}
        \caption{}
        \label{fig:NYC_full_net}
    \end{subfigure}
    \caption{(a) All available road segments in the road map of Eastern Massachusetts, (b) New York network with speed data (February 13, 2019 at 9:00 a.m.) retrieved from Uber Movement. }
    \label{fig:full_net}
\end{figure}
